# Supplementary material for: Grounded Human-Object Interaction Hotspots from Video (Extended Abstract)
Source: arXiv:1906.01963 source file (2019-06-03)
Supplement: Supplementary file 1 [file supp.tex]

\newpage

\setcounter{section}{0}
\setcounter{figure}{0}
\setcounter{table}{0}

\section*{Supplementary Material}

This section contains supplementary material to support the main paper text. The contents include:
\begin{itemize}[leftmargin=*]
\itemsep0em 
    \item (\S\ref{sec:videos}) A video demonstrating our method on clips of human-object interaction.
    \item (\S\ref{sec:ablation}) Ablation study of our model components in \refsec{sec:distill} and \refsec{sec:hotspot_modifications} of the main paper.
    \item (\S\ref{sec:annotation}) EPIC Kitchens data annotation details. 
    \item (\S\ref{sec:l_ant}) Details about the anticipation loss $\mathcal{L}_{ant}$ for EPIC Kitchens described in \refsec{sec:exp} (Datasets).      
    \item (\S\ref{sec:implementation}) Implementation details for our model and experiments in \refsec{sec:grounded-affordances}.
    \item (\S\ref{sec:img2heatmap}) Architecture details for the \SC{Img2heatmap} model introduced in \refsec{sec:grounded-affordances} (Baselines)
    \item (\S\ref{sec:evaluation}) Additional details about the evaluation protocol for our experiments in \refsec{sec:grounded-affordances}.
    \item (\S\ref{sec:examples}) More examples of hotspot predictions on OPRA and EPIC to supplement \reffig{fig:opra-qual} in the main paper.
    \item (\S\ref{sec:clustering}) Clustering visualizations to accompany the results in \refsec{sec:dendo}.
\end{itemize}

\section{Interaction hotspots generated on video clips} \label{sec:videos}
We demonstrate our method on videos from EPIC by computing hotspots for each frame of a video clip. Note that the OPRA test set consists only of static images (\reftbl{tbl:hotspot-eval} in main paper), as following the evaluation protocol in \cite{fang2018demo2vec}. The video can be found on the \href{http://vision.cs.utexas.edu/projects/interaction-hotspots/}{project page}. Our model is trained on all actions, but we show hotspots for 5 frequent actions (cut, mix, adjust, open and wash) for clarity. Our model is able to derive hotspot maps on inactive objects \emph{before} the interaction takes place. During this time, the objects are at rest, and are not being interacted with, yet our model can anticipate how they could be interacted with. In contrast to prior weakly supervised saliency methods, our model generates distinct maps for each action that aligns with object function. Some failure modes include when our model is presented rare objects/actions or unfamiliar viewpoints, for which our model produces diffused or noisy heatmaps.

\begin{table}[t]
\centering
\resizebox{\columnwidth}{!}{
\begin{tabular}{l|ccc|ccc}
\multicolumn{1}{c}{}                &          \multicolumn{3}{c}{OPRA}                    &           \multicolumn{3}{c}{EPIC}                   \\
\cmidrule(l{2pt}r{2pt}){2-4} \cmidrule(l{2pt}r{2pt}){5-7}
                                    & KLD $\downarrow$ & SIM $\uparrow$ & AUC-J $\uparrow$ & KLD $\downarrow$ & SIM $\uparrow$ & AUC-J $\uparrow$ \\
\cmidrule{1-7}
\SC{Ours (basic)}                   & 1.561            & 0.349          & 0.707            & 1.342           & 0.396          & 0.714             \\
\SC{+ Resolution}                   & 1.492            & 0.352          & 0.766            & 1.343           & 0.395          & 0.731             \\ 
\SC{+ L2 pool}                      & 1.489            & 0.349          & 0.770            & 1.361           & 0.385          & 0.727             \\
\SC{+ Anticipation}                 & \B{1.427}        & \B{0.362}      & \B{0.806}        & \B{1.258}       & \B{0.404}      & \B{0.785}         \\
\cmidrule{1-7}
\end{tabular}
}
\caption{\textbf{Ablation study of model enhancements}. Using a larger backbone feature resolution, L2-pooling, and the anticipation module improves our model performance, and are essential for well localized hotspot maps.
} 
\label{tbl:ablation}
\end{table}

\section{Ablation study} \label{sec:ablation}
As noted in the main paper (\refsec{sec:grounded-affordances}), we study the effect of each proposed component in \refsec{sec:distill} and \refsec{sec:hotspot_modifications} on the performance of our model. \reftbl{tbl:ablation} shows how they contribute towards more affordance aware activation maps. Specifically, we see that increasing the backbone resolution to N=28 increases AUC-J from 0.707 to 0.766. Using L2-pooling to ensure that spatial locations produce gradients as a function of their activation magnitudes increases this to 0.770, and using our anticipation model (\refsec{sec:distill} of the main paper) further increases AUC-J to \textbf{0.806}.
Note that within our model, hotspots \emph{could} be be derived at the output hypothesized image, corresponding to hotspots on a regular video frame, but this does not align with the static images, causing a drop in performance (0.806 vs. 0.723 AUC-J). Propagating gradients back through the anticipation module produces correctly aligned gradients. 
More generally, we observe consistent improvement for our components across all metrics on both OPRA and EPIC.

\section{Data collection setup for EPIC-Kitchens annotations} \label{sec:annotation}
As mentioned in \refsec{sec:exp} (Datasets), we collect annotations for interaction keypoints on EPIC Kitchens in order to quantitatively evaluate our method in parallel to the OPRA dataset (where annotations are available). We note that these annotations are collected purely for evaluation, and are not used for training our model. We select the 20 most frequent verbs, and select 31 nouns that afford these interactions. The list of verbs and nouns can be found in \reftbl{tbl:verb_noun_subset}. To select instances for annotation, we first identify frames in the EPIC Kitchen videos which contain the object, and crop out the object using the provided bounding box annotations. Most of these object crops are \emph{active} \ie the objects are not at rest and/or they are being actively manipulated. We discard instances where hands are present in the crop using an off the shelf hand detection model, and manually select for 
\emph{inactive} images from the remaining object crops. These images are then annotated.

\begin{figure}[t!]
\centering
\includegraphics[width=\linewidth]{figures/mturk}
\caption{\textbf{Interface for collecting annotations on EPIC.} Users are asked to watch a video containing an interaction, and mark keypoints at the location of the interaction.}
\label{fig:mturk}
\end{figure}

We crowdsource these annotations using the Amazon Mechanical Turk platform. Following \cite{fang2018demo2vec}, our annotation setup is as follows. A user is asked to watch a short video (2-5s) of an object interaction (eg. person cutting carrot), and place 1-2 points on an image of the object for where the interaction is performed. We solicited 5 annotations for the same image (from unique users) to account for inter-annotator variance. Overall, we collected 19800 responses from 613 workers for our task, resulting in 1871 annotated (image, verb) pairs. Our annotation interface is shown in \reffig{fig:mturk}.

Finally, following~\cite{fang2018demo2vec}, we convert these annotations into a heatmap by centering a gaussian distribution over each point. We use this heatmap as our ground truth $\mathcal{M}$ described in \refsec{sec:exp} (Datasets). Some examples of these collected annotations and their correspondingly derived heatmaps are shown in \reffig{fig:annotations}.

\begin{table}[t!]
\centering
\resizebox{\columnwidth}{!}{
\begin{tabular}{|p{1cm}|p{8cm}|} \hline
\B{verbs} & take, put, open, close, wash, cut, mix, pour, throw, move, remove, dry, turn-on, turn, shake, turn-off, peel, adjust, empty, scoop \\ \hline
\B{nouns} & board:chopping, bottle, bowl, box, carrot, colander, container, cup, cupboard, dishwasher, drawer, fork, fridge, hob, jar, kettle, knife, ladle, lid, liquid:washing, microwave, pan, peeler:potato, plate, sausage, scissors, spatula, spoon, tap, tongs, tray \\ \hline
\end{tabular} 
}
\caption{Verbs and nouns annotated for EPIC.}
 \label{tbl:verb_noun_subset}
\end{table}

Compared to asking annotators to label static images with affordance labels (\eg, label "openable"), annotations collected by watching videos and then placing points is well-aligned with our objective of learning fine-grained object interaction. The annotations are better localized and are grounded in real human demonstration, making them meaningful for evaluation.

\section{Anticipation loss for EPIC-Kitchens} \label{sec:l_ant}
As mentioned in \refsec{sec:distill} and \refsec{sec:hotspot_modifications}, we require inactive images to train the anticipation model. For OPRA, these are the catalog photos of the object provided with each video. In EPIC, we crop out inactive objects from frames using the provided bounding boxes $\mathcal{B}$, and select the inactive image that has the same class label as the object in the video. Unlike OPRA, these images may be visually different from the object in the video, preventing us from using the L2 loss directly. Instead, we use a triplet loss for the anticipation loss term as follows:
\begin{equation*}
    \begin{split}
    \mathcal{L}^\prime_{ant}(\mathcal{V}, x_{I}, x_{I'}) =  \max \left [
        0, d(P(x_{t^*}), P(\widetilde{x}_I) \right. \\
        \left. - d(P(x_{t^*}), P(\widetilde{x}_{I'})) + M \right ],
    \end{split}
\label{eq:triplet}
\end{equation*}
where $x_I$ and $x_{I'}$ represent inactive image features with the correct and incorrect object class respectively. $d$ denotes Euclidean distance, and $M$ is the margin value. We normalize the inputs before computing the triplet loss, thus we keep the margin value fixed at 0.5. This term ensures that inactive objects of the correct class can anticipate active features better than incorrect classes, and is less sensitive to appearance mismatches compared to \refeqn{eqn:anticipation} in the main paper.

\begin{figure}[t!]
\centering
\includegraphics[width=\linewidth]{figures/annotations}
\caption{\textbf{Top:} Some example annotations provided as keypoints on EPIC object crops \textbf{Bottom:} The resulting heatmaps derived from these annotations, to be used as ground truth for evaluation.}
\label{fig:annotations}
\end{figure}

\begin{figure*}[t!]
\centering
\includegraphics[width=\linewidth]{figures/dendo}
\caption{\textbf{Clustering of the average object embedding in the appearance vs. interaction hotspot feature space.} Appearance features capture similarities in shapes and textures (knife, tongs) and object co-occurrence (pan, lid; cup, kettle). In contrast, our interaction hotspot features encode similarities that are aligned with object function and use (cupboard, microwave, fridge - characteristically swung open; carrot, sausage - cut and held similarly). Similarity in this space refers to L2 distance between average object embeddings.}
\label{fig:dendograms}
\end{figure*}

\section{Implementation details} \label{sec:implementation}
We provide implementation and training details for our experiments in  \refsec{sec:exp}. For all experiments, we use an ImageNet~\cite{krizhevsky2012imagenet} pretrained ResNet-50~\cite{he2016deep} modified for higher output resolution. To increase the output dimension from $n = 7 $ to $n = 28$, we set the spatial stride of res$_4$ and res$_5$ to 1 (instead of 2), and use dilation of 2 (res$_4$) and 4 (res$_5$) for its filters to preserve the original scale.  For $\mathcal{F}_{ant}$ we use 2 sets of  (conv-bn-relu) blocks, with 3x3 convolutions, maintaining the channel dimension $d=2048$. We use a single layer LSTM (hidden size 2048) as $\mathbb{A}$, and train using chunks of 16 frames at a time. For our combined loss (\refeqn{eqn:total_loss} in the main paper), we set $\lambda_{cls} = \lambda_{aux} = 1$ and $\lambda_{ant} = 0.1$ based on validation experiments. Our models are implemented in PyTorch. Adam with learning rate 1e-4, weight decay 5e-4 and batch size $128$ is used to optimize the models parameters.

\section{Architecture details for supervised baselines} \label{sec:img2heatmap}
The \SC{Img2heatmap} model in \refsec{sec:grounded-affordances} is a fully convolutional encoder-decoder to predict the affordance heatmap for an image. The encoder is an ImageNet pretrained VGG16 backbone (up to conv5), resulting in an encoded feature with 512 channels and spatial extent 7. This feature is passed through a decoder with an architecture mirroring the backbone, where the max-pooling operations are replaced with bilinear upsampling operations. This results in an output of the same dimension as the input, and as many channels as the number of actions. The output of this network is fed through a sigmoid operator and reconstruction loss against the ground truth affordance heatmap is calculated using binary cross-entropy.

\section{Evaluation protocol for grounded affordance prediction} \label{sec:evaluation}
As discussed in \refsec{sec:grounded-affordances}, the heatmaps generated by our model and the baselines are evaluated against the manually annotated ground truth heatmaps provided in the OPRA dataset and collected on EPIC (results in \reftbl{tbl:hotspot-eval}). For a single action (\eg ``press" a button), the ground truth heatmaps may occur distributed across several instances (\eg different clips of people pressing different buttons on the same object). We simply take the union of all these heatmaps as our target affordance heatmap for the action. For evaluation, this leaves us with 1042 (image, action) pairs in OPRA, and 571 (image, action) pairs in EPIC. For AUC-J, we binarize heatmaps using a threshold of $0.5$ for evaluation.

\section{Additional examples of generated hotspot maps} \label{sec:examples}
We provide more examples of our hotspot maps to accompany our results in the main paper. \reffig{fig:opra-supp} and \reffig{fig:epic-supp} contains more examples of these on OPRA and EPIC respectively to supplement our results in \reffig{fig:opra-qual} in the main paper. Unlike the baselines, our model highlights multiple distinct affordances for an object and does so without heatmap annotations during training. The last 4 images in each figure show some failure cases where our model is unable to produce heatmaps for small or unfamiliar objects. 

\section{Clustering visualization for appearance vs. our interaction hotspot features} \label{sec:clustering}
We show the full clustering of objects in the appearance vs. interaction hotspot feature space to supplement the nearest neighbor visualizations presented in \refsec{sec:dendo} of the main paper. Each object is represented by a vector obtained by averaging the embeddings of all instances for that specific object class. The resultant \emph{average object representations} for all classes are then clustered using agglomerative hierarchical clustering. L2 distance in this space represents average similarity between object classes. 

\reffig{fig:dendograms} shows how our learned representation groups together objects related by their function and interaction modality, more so than the original appearance-based visual representation. Appearance features capture similarities in shapes and textures (knife, tongs) and object co-occurrence (pan, lid; cup, kettle). In contrast our representation encodes object function. Cupboards, microwaves, fridges that are characteristically swung opened; knives and scissors that afford the same cutting action; carrots, sausages that are cut and held in the same manner, are clustered together.

\begin{figure*}[t!]
\centering
\includegraphics[width=\linewidth]{figures/opra-supp}
\caption{\textbf{Generated affordance heatmaps on inactive images from OPRA.} Our interaction hotspot maps show holdable, rotatable, and pushable regions (in red, green, and blue respectively). Saliency heatmaps do not discriminate between interactions and produce a single heatmap shown in yellow. Recall that the \SC{demo2vec} approach~\cite{fang2018demo2vec} is strongly supervised, whereas our approach is weakly supervised. Some failure cases due to small or unfamiliar objects can be seen in the last 4 examples.}
\label{fig:opra-supp}
\end{figure*}

\begin{figure*}[t!]
\centering
\includegraphics[width=\linewidth]{figures/epic-supp}
\caption{\textbf{Generated interaction hotspot maps on inactive images from EPIC-Kitchens.} Our interaction hotspot maps show cuttable, mixable, adjustable, and openable regions (in red, green, blue, and cyan, respectively). Failure cases can be seen in the last 4 examples.}
\label{fig:epic-supp}
\end{figure*}
